# Supplementary material for: Josephson anomalous vortices
Source: arXiv:2504.17779 ancillary file (2025-10-10)
Supplement: Supplementary file 1 [file SI-josephson-anomalous-vortices.pdf]

# Supplemental Material: Josephson anomalous vortices

Dan Crawford,[1] Stefan Ilić,[1] Pauli Virtanen,[1] and Tero T. Heikkilä[1]
[1]*Department of Physics and Nanoscience Center, University of Jyväskylä, P.O. Box 35 (YFL), FI-40014 University of Jyväskylä, Finland*
(Dated: April 24, 2025)

## CONTENTS

I. Nonlinear $\sigma$ model and magnetoelectric effects 1
II. Invariants with linear-in-momentum spin-orbit coupling 2
III. Vortex phase transition as a function of spin-orbit coupling and system size 4
IV. Josephson current in the presence of the rotary invariant 4
References 5

## I. NONLINEAR $\sigma$ MODEL AND MAGNETOELECTRIC EFFECTS

In this section, we review the microscopic model. A generic superconducting system including spin-orbit coupling and magnetism is described by the Hamiltonian

$$H = \tau_3 \left[ \frac{(\boldsymbol{k} - \check{\boldsymbol{A}}(\boldsymbol{r}))^2}{2m} - \mu + V_{\rm imp}(\boldsymbol{r}) - \check{A}_0(\boldsymbol{r}) \right] + \hat{\Delta}(\boldsymbol{r}). \tag{1}$$

Here $\boldsymbol{k}$ is the momentum for an electron with mass $m$ at chemical potential $\mu$. $V_{\rm imp}$ is a random impurity potential. $\check{\boldsymbol{A}}$ captures the $U(1)$ scalar ($\Phi$) and vector ($A_i$) electromagnetic potentials, and the $SU(2)$ linear-in-momentum spin-orbit coupling ($\boldsymbol{\mathcal{A}}_\mu$), with $\check{A}_i = A_i\tau_3 + \boldsymbol{\mathcal{A}}_i \cdot \boldsymbol{\sigma}$ and $\check{A}_0 = \Phi + \boldsymbol{\mathcal{A}}_0 \cdot \boldsymbol{\sigma}\tau_3$ $\hat{\Delta} = \tau_1\sigma_0\Delta(\boldsymbol{r})e^{i\tau_3\varphi}$ is the superconducting pair potential. We assume that the variance of $V_{\rm imp}$ is large and the system is in the diffusive transport regime, where the mean free path $\ell$ is much longer than the Fermi wavelength $\lambda_{\rm F} = k_{\rm F}^{-1}$, but much smaller than the coherence length, $\xi_0 \gg \ell \gg \lambda_{\rm F}$. We use the conventions that Greek subscripts $\mu, \nu$ run over $(0, 1, 2, 3)$, while Latin subscripts run over $(1, 2, 3)$. $\tau_\mu$ are Pauli matrices in particle-hole space and $\sigma_\mu$ are Pauli matrices in spin space. Products of $\tau_\mu$ and $\sigma_\mu$ are Kronecker products.

The disorder-averaged physics of this model is described by the action [1, 2].

$$S[Q] = S_{0,1}[Q] + S_{0,2}[Q] + S_{\rm rot}[Q], \tag{2}$$

$$S_{0,1}[Q] = \hbar\frac{i\pi\nu_{\rm F}}{8}{\rm Tr}[D(\check{\nabla}Q)^2], \tag{3}$$

$$S_{0,2}[Q] = \frac{i\pi\nu_{\rm F}}{8}{\rm Tr}[4i\Omega Q], \tag{4}$$

$$S_{\rm rot}[Q] = \hbar\frac{i\pi\nu_{\rm F}}{8}{\rm Tr}[\eta\check{F}_{ij}Q\check{\nabla}_iQ\check{\nabla}_jQ]. \tag{5}$$

Here we have the density of states per spin at the Fermi level $\nu_{\rm F}$ and $\eta = D\ell^2/(k_{\rm F}\ell)$. The diffusion constant is $D = v_{\rm F}^2\tau/2 = v_{\rm F}\ell/2$, with $v_{\rm F}$ the Fermi velocity and $\tau$ the elastic scattering time. The prefactor $\eta$ can also be expressed in terms of the Dyakonov–Perel rate $\Gamma_r = 4D\alpha^2$ and the spin-triplet conversion rate $\Gamma_{st} = (\hbar^3\Gamma_r^3\Delta_0)^{1/2}/(2\hbar E_F)$ as $\hbar\eta = \frac{\hbar\Gamma_{st}\Delta_0^{1/2}}{(\hbar\Gamma_r)^{3/2}} \times \Delta_0\xi_0^4$, where $\Delta_0$ is the zero-temperature singlet superconducting gap and $\xi_0 = \sqrt{\hbar D/\Delta_0}$ the corresponding coherence length. In all numerical results, we assume $\hbar\eta = 0.01\Delta_0\xi_0^4$. For numerics, we work in natural units $e = \hbar = k_{\rm B} = 1$, and use $\xi_0$ and $\Delta_0$ as the natural length and energy units. We use the covariant derivative $\check{\nabla}_i = \partial_i \cdot -i[\check{A}_i, \cdot]$ and $\Omega = i\varepsilon\sigma_0\tau_3 + \hat{\Delta}(\boldsymbol{r}) + \check{A}_0\tau_3$. The field strength tensor is

$$\check{F}_{\mu\nu} = \partial_\mu\check{A}_\nu - \partial_\nu\check{A}_\mu - i[\check{A}_\mu, \check{A}_\nu]. \tag{6}$$

The matrix current is given by derivatives of this action

$$\mathcal{J}_\mu = \frac{2i}{\pi\nu_\mathrm{F}}\frac{\delta S}{\delta \check{A}_\mu}. \tag{7}$$

The charge current is computed from the matrix current as

$$J_i^c = -e\frac{\pi\nu_\mathrm{F}}{2}\mathrm{Tr}\tau_3\mathcal{J}_i. \tag{8}$$

Assuming weak superconductivity, this action can be linearized by

$$Q \approx \begin{pmatrix} 1-\frac{1}{2}f\bar{f} & f \\ \bar{f} & -1+\frac{1}{2}\bar{f}f \end{pmatrix}, \tag{9}$$

with the superconducting correlations $f = f_s + \boldsymbol{f}_t\cdot\boldsymbol{\sigma}$, and $\bar{f} = \sigma_y f^* \sigma_y = f_s^* - \boldsymbol{f}_t^*\cdot\boldsymbol{\sigma}$. We proceed by assuming there is a general exchange field $\boldsymbol{\mathcal{A}}_0 = (h_x, h_y, h_z)$, and Rashba spin-orbit coupling $\boldsymbol{\mathcal{A}}_i = (\alpha, -\alpha, 0)$. Substituting these into Eq. (2) yields the following linear action:

$$S = i\pi\nu_\mathrm{F}(S_{0,1} + S_{0,2} + S_\mathrm{rot}) + \mathrm{c.c.},$$

$$S_{0,1} = \hbar D\Big[i(A_x f_\mu^* \partial_x f_\mu + A_y f_\mu^*\partial_y f_\mu) + i\alpha(-f_s\partial_x f_y^* + f_y \partial_x f_s^* + f_s\partial_y f_x^* - f_x\partial_y f_s^*) + 2\alpha(-A_x f_x f_y^* + A_y f_x f_y^*)\Big], \tag{10}$$

$$S_{0,2} = \Big[\left(\Delta f_y - \Delta f_y^*\right) - 2i\Phi - 2i\varepsilon + i(\Phi+\varepsilon)f_\mu f_\mu^* + (ih_x f_s f_x^* + h_y f_x f_z^* + ih_z f_s f_z^*)\Big], \tag{11}$$

$$S_\mathrm{rot} = \hbar\eta\Big[\alpha^2\left(\hat{\nabla} f_s \times \hat{\nabla}^* f_z^*)\cdot\hat{z}\right) + 2\alpha^3\left((\boldsymbol{f}_t\times\hat{\nabla} f_s^*)\cdot\hat{z}\right)\Big]. \tag{12}$$

Here we use $\hat{\nabla} = (\partial_x \cdot + 2iA_x\cdot, \partial_y \cdot - 2iA_y, 0)$. In $S_\mathrm{rot}$ the term proportional to $\alpha^3$ is the Lifshitz invariant, while the rotary invariant is proportional to $\alpha^2$. This yields the following charge current density

$$\boldsymbol{J}_{0,1} = i\pi\nu_\mathrm{F}\hbar e D\left(f_\mu \hat{\nabla} f_\mu^* + \mathrm{c.c.}\right) \tag{13}$$

$$\boldsymbol{J}_\mathrm{rot} = i\pi\nu_\mathrm{F}\hbar e\eta\left(2\alpha^2(f_s \mathrm{curl} f_z^* + f_z\mathrm{curl} f_s^*) + 4\alpha^3(f_j^* f_z - f_j f_z^*)\right). \tag{14}$$

Here $\mathrm{curl}\,A = (\partial_y A, -\partial_x A)$ and $f_j = (f_x, f_y)$. The term proportional to $\alpha^3$ is due to the Lifshitz invariant, while the rotary invariant is proportional to $\alpha^2$. $\boldsymbol{J}_{0,1}$ is the conventional supercurrent.

## II. INVARIANTS WITH LINEAR-IN-MOMENTUM SPIN-ORBIT COUPLING

In this section, we derive the Lifshitz and rotary invariants from the microscopic theory for general linear-in-momentum SOC, and also the corresponding terms in the Ginzburg–Landau expansion. Let us denote with $\mathcal{F}_\mathrm{me}$ the part of the free energy of the superconductor that describes magnetoelectric phenomena. It comes from the $S_\mathrm{rot}$ contribution in the $\sigma$ model action, and in the Matsubara representation it has the form

$$\mathcal{F}_\mathrm{me} = -\frac{\pi T}{16}\sigma'_{xy}\sum_{\omega_n}\mathrm{Tr}[\check{F}_{ij} Q\check{\nabla}_i Q\check{\nabla}_j Q]. \tag{15}$$

Here, $\sigma'_{xy} = 2\nu_\mathrm{F}\eta$ is the zero-field derivative of the Hall conductivity and Tr stands for the trace in Nambu and spin space. As above, we focus on the Ginzburg-Landau regime, where superconductivity is weak and we can approximate using Eq. (9). Substituting this form of $Q$ into the expression for $\mathcal{F}_\mathrm{me}$ while keeping terms up to the second order in $f$ yields

$$\mathcal{F}_\mathrm{me} = -\frac{\pi T}{16}\sigma'_{xy}\sum_{\omega_n}\mathrm{Tr}[F_{ij}\tau_3\check{\nabla}_i(f\tau_+ + \bar{f}\tau_-)\check{\nabla}_j(f\tau_+ + \bar{f}\tau_-)], \tag{16}$$

where $\tau_\pm = \frac{1}{2}(\tau_1 \pm i\tau_2)$. Next, we assume that the applied Zeeman field is weak, and we consider only terms up to the first order in $h_k$. Since in this regime $f_k \propto h_k$, we may keep only terms up to first order in triplet correlations $f_k$. This gives

$$\mathcal{F}_\mathrm{me} = -\frac{\pi T}{8}\sigma'_{xy}\sum_{\omega_n}\mathrm{Tr}_\sigma[F_{ij}\sigma_k](\Pi_i f_s \Pi_j^*\bar{f}_k - \Pi_i^*\bar{f}_s\Pi_j f_k) - \frac{\pi T}{8}\sigma'_{xy}\sum_{\omega_n}\mathrm{Tr}_\sigma[F_{ij}[\mathcal{A}_j,\sigma_k]](\Pi_i f_s\bar{f}_k + \Pi_i^*\bar{f}_s f_k). \tag{17}$$

Here, $\mathrm{Tr}_\sigma$ stands for the trace in spin space and the momentum is $\Pi_i = -i\hbar\partial_i - 2A_i$.

The free-energy functional for the superconducting order parameter $\psi(\boldsymbol{r})$ is obtained by finding the saddle point of the total functional $F[\psi, Q]$ with respect to $Q$. [3] To obtain the Ginzburg-Landau theory perturbatively in gradients, it is sufficient to use the saddle point of the gradient-free part of the functional, which corresponds to finding the anomalous Green's function $f$ from the homogeneous linearized Usadel equation for given $\psi(\boldsymbol{r})$. The solution in general has the form $f(\boldsymbol{r}) = \psi(\boldsymbol{r})(\tilde{f}_s + i\tilde{f}_k\sigma_k)$. The functions $\tilde{f}_s$ and $\tilde{f}_k$ are real, so that $\bar{f}(\boldsymbol{r}) = \psi^*(\boldsymbol{r})(\tilde{f}_s + i\tilde{f}_i\sigma_i)$. The magnetoelectric part of the free energy now becomes

$$\mathcal{F}_{\mathrm{an}} = ie_{ij}\Pi_i\psi(\Pi_j\psi)^* + d_i(\psi^*\Pi_i\psi + \psi(\Pi_i\psi)^*), \tag{18}$$

where we introduced the rotary invariant

$$e_{ij} = -\frac{\pi T}{8}\sigma'_{xy}\mathrm{Tr}_\sigma[F_{ij}\sigma_k]\sum_{\omega_n}\tilde{f}_s\tilde{f}_k, \tag{19}$$

and the Lifshitz invariant

$$d_i = -\frac{i\pi T}{8}\sigma'_{xy}\mathrm{Tr}_\sigma[F_{ij}[\mathcal{A}_j, \sigma_k]]\sum_{\omega_n}\tilde{f}_s\tilde{f}_k. \tag{20}$$

We next neglect the relaxation of triplet correlations $f_k$, so that $\tilde{f}_s = \omega_n/(\omega_n^2 + h^2) \approx 1/\omega_n$ and $\tilde{f}_k = h_k/(\omega_n^2 + h^2) \approx h_k/\omega_n^2$. We explicitly perform the summation over Matsubara frequencies using $2\pi T\sum_{\omega_n>0} 1/\omega_n^3 = 7\zeta(3)/(4\pi^2 T_c^2)$, where $\zeta(n)$ is the Zeta function and the expression is valid when the temperature is close to the critical temperature $T \approx T_c$. Finally, the rotary and Lifshitz invariants are

$$e_{ij} = -\frac{\sigma'_{xy}}{8}\frac{7\zeta(3)}{4\pi^2 T_c^2}\mathrm{Tr}_\sigma[F_{ij}\sigma_k h_k], \qquad d_i = -\frac{i\sigma'_{xy}}{8}\frac{7\zeta(3)}{4\pi^2 T_c^2}\mathrm{Tr}_\sigma[F_{ij}[\mathcal{A}_j, \sigma_k h_k]]. \tag{21}$$

Defining

$$\kappa = -\frac{\sigma'_{xy}}{8}\frac{7\zeta(3)}{4\pi^2 T_c^2} \tag{22}$$

then yields the expressions, Eq. (2), in the main text.

We can carry out the corresponding calculation for the gradient energy term described by the action $S_{0,1}$ to obtain the $D_S$ term of the Ginzburg-Landau theory. For an order-of-magnitude estimate, we concentrate only on the $\alpha = 0$ term. This yields

$$D_S = \frac{\pi T\nu_F D}{2}\sum_{\omega_n} f_s^2 = \frac{\pi T\nu_F D}{2}\sum_{\omega_n}\frac{1}{\omega_n^2} = \frac{\pi\nu_F D}{8T_c}. \tag{23}$$

In other words, in a Rashba model with $F_{xy} = 2\alpha^2\sigma_z$ and with $\mathbf{h} = h\hat{u}_z$, we get

$$\frac{\epsilon_{xy}}{D_S} = \frac{7\zeta(3)}{4\pi^3}\frac{\alpha^2\ell^2}{k_F\ell}\frac{h}{T_c}. \tag{24}$$

Since the prefactor is much below unity, the exchange field $h$ usually cannot be much larger than $T_c$ without breaking superconductivity, and the quasiclassical diffusive model assumes $\alpha\ell \ll 1$ and $k_F\ell \gg 1$, this approach ceases to be valid for $\epsilon_{xy} \sim D_S$, required for the vortex transition in a bulk superconductor (see Eq. (16) in the main text). However, as shown in the main text, the transition to the vortex state in a Josephson junction is within the validity range of the quasiclassical diffusive limit theory. Nevertheless, the phenomenological model does not rely on similar assumptions as the quasiclassical theory, so its qualitative predictions remain valid.

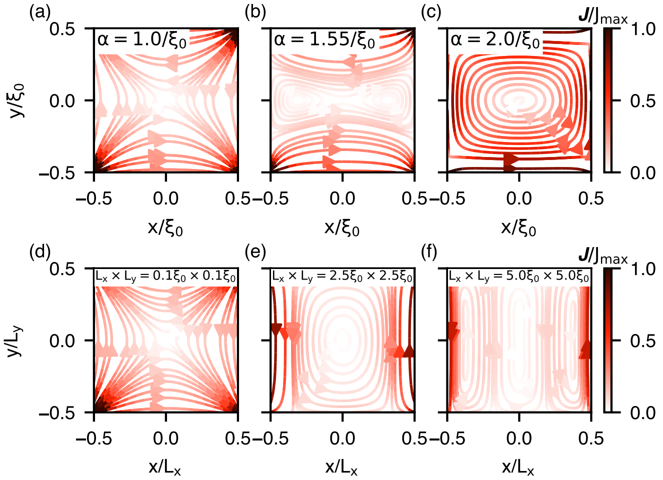


FIG. 1. (abc) Current densities as a function of $\alpha$, highlighting the antivortex (a), transitional (b), and vortex (c) phases. Parameters: $(L_x, L_y, J) = (\xi_0, \xi_0, \Delta_0)$. (d-f) Current densities as a function of system size. Parameters: $(\alpha, J) = (2/\xi_0, \Delta_0)$.

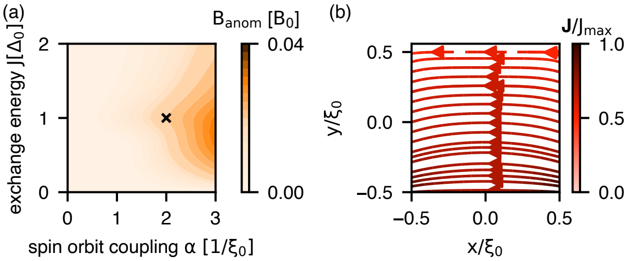


FIG. 2. (a) Magnetic flux due to swirling currents at finite phase bias $\varphi = (2/3)\pi$. $B_0$ is defined in the main text. (b) Current density at the point marked by × in (a). Parameters: $(L_x, L_y) = (\xi_0, \xi_0)$.

## III. VORTEX PHASE TRANSITION AS A FUNCTION OF SPIN-ORBIT COUPLING AND SYSTEM SIZE

In Fig. 1(a-c) we show the current densities for a range of $\alpha$ with $J = \Delta_0$ fixed, and system size $L_x \times L_y = \xi_0 \times \xi_0$. For $\alpha = 1/\xi_0$ we see a representative antivortex. For $\alpha = 2/\xi_0$ we see a representative vortex. In between, at $\alpha = 1.55/\xi_0$, the system is in a transitional phase. The currents along the terminals have been "pinched off" to form two copropagating vortices. As $\alpha$ increases, these vortices merge and fill the weak link. As seen in Fig. 2 of the main text, these copropagating vortices can be robust over a large range of $\alpha, J$, resulting in large parts of parameter space in this transitional phase. In Fig. 1(d-f) we plot the current density for fixed $(\alpha, J) = (2/\xi_0, \Delta_0)$ and varying system sizes. As noted in the main text, for small junctions parameter space is dominated by antivortices. For large junctions counterpropagating current loops form close to the superconducting terminals due to triplet oscillations [4], while a weak JAV is squeezed in the center. These counterpropagating loops produce a magnetic flux with the opposite sign to the central vortex, resulting in a tiny overall magnetic flux. For intermediate sized junctions, a central vortex can appear, with minimal effects due to the terminals.

## IV. JOSEPHSON CURRENT IN THE PRESENCE OF THE ROTARY INVARIANT

In Fig. 2(a) we plot the magnetic field at the center of the junction for finite phase bias $\varphi = (2/3)\pi$. While at zero phase bias there is a large magnetic field around $J = 1, \alpha = 2$ (see Fig. 2 in the main text), here there is a much smaller flux. The rotary invariant Eq. (12) applies a small perturbation to the usual Josephson current Eq. (10), resulting in a "bending" of the current (Fig. 2(b)), as opposed to the usual straight left-to-right charge transport across an SNS

junction.

[1] P. Virtanen, F. S. Bergeret, and I. V. Tokatly, Phys. Rev. B **105**, 224517 (2022).
[2] P. Virtanen, F. S. Bergeret, and I. V. Tokatly, Phys. Rev. B **104**, 064515 (2021).
[3] P. Virtanen, Phys. Rev. B **111**, 024510 (2025).
[4] F. S. Bergeret, A. F. Volkov, and K. B. Efetov, Rev. Mod. Phys. **77**, 1321 (2005).
